# Supplementary material for: Efficient Architecture Search via Bi-level Data Pruning
Source: arXiv:2312.14200 source file (2023-12-21)
Supplement: Supplementary file 1 [file X_suppl.tex]

\clearpage
\setcounter{page}{1}
\maketitlesupplementary

\setcounter{section}{0}
\setcounter{figure}{0}
\setcounter{table}{0}

 % 使用字母编号

This appendix further provides additional experiments and details (including comparisons of detailed searching trajectory, effectiveness verification of the class balance constraint, comparisons of different class balance constraints, details of data pruning strategy), the visualization of the searched architectures (including DARTS and Mobile search spaces), and a discussion of limitations.
% several additional experiments (the training trajectories of DARTS and DARTS w/ BDP, the effect of class balance constraint, and the comparison of different class balance constraints) (~\cref{sec: appendix: additional exps}), an effectiveness analysis of BDP from Hessian matrix (~\cref{sec: appendix: analysis of Hessian}), more details of data pruning strategies combination experiments (~\cref{sec: appendix: combinations}), and the visualization of the searched architectures of DARTS and DARTS w/ BDP on DARTS search space(~\cref{sec: appendix: cell structure}).

\section{Additional Experiments and Details}
\label{sec: appendix: additional exps}

\subsection{Detailed Searching Trajectory Comparisons}
\label{sec: appendix: trajectories}
Firstly,~\cref{fig: bench_change_C10} and ~\cref{fig: bench_change_C100} show more searching trajectory comparisons of DARTS w/ BDP and DARTS~\cite{liu2018darts} when searching on CIFAR-10 and CIFAR-100 datasets on the NAS-Bench-201 benchmark~\cite{dong2020bench}, respectively. From subgraphs (a), (b), and (c) of each figure, we can see that DARTS w/ BDP outperforms DARTS on all test datasets for almost the whole searching period. More importantly,  we can see that DARTS w/ BDP can achieve high performance in the early stage of training (before 20 epochs) on both CIFAR-10 and CIFAR-100 datasets. And the performance can be maintained in the subsequent training process. In addition, as shown in subgraphs (d), the number of samples of DARTS w/ BDP consistently decreases, resulting in improved training efficiency. Subgraphs (f) show that BDP can suppress the problem of continuous increase of the Hessian norm of DARTS, therefore obtaining better architectures. The analysis of the effectiveness from the Hessiam norm is discussed in ~\cref{sec: effectiveness analysis}. 

\begin{figure*}[htbp] 
	\centering 
	\includegraphics[width=0.86\linewidth]{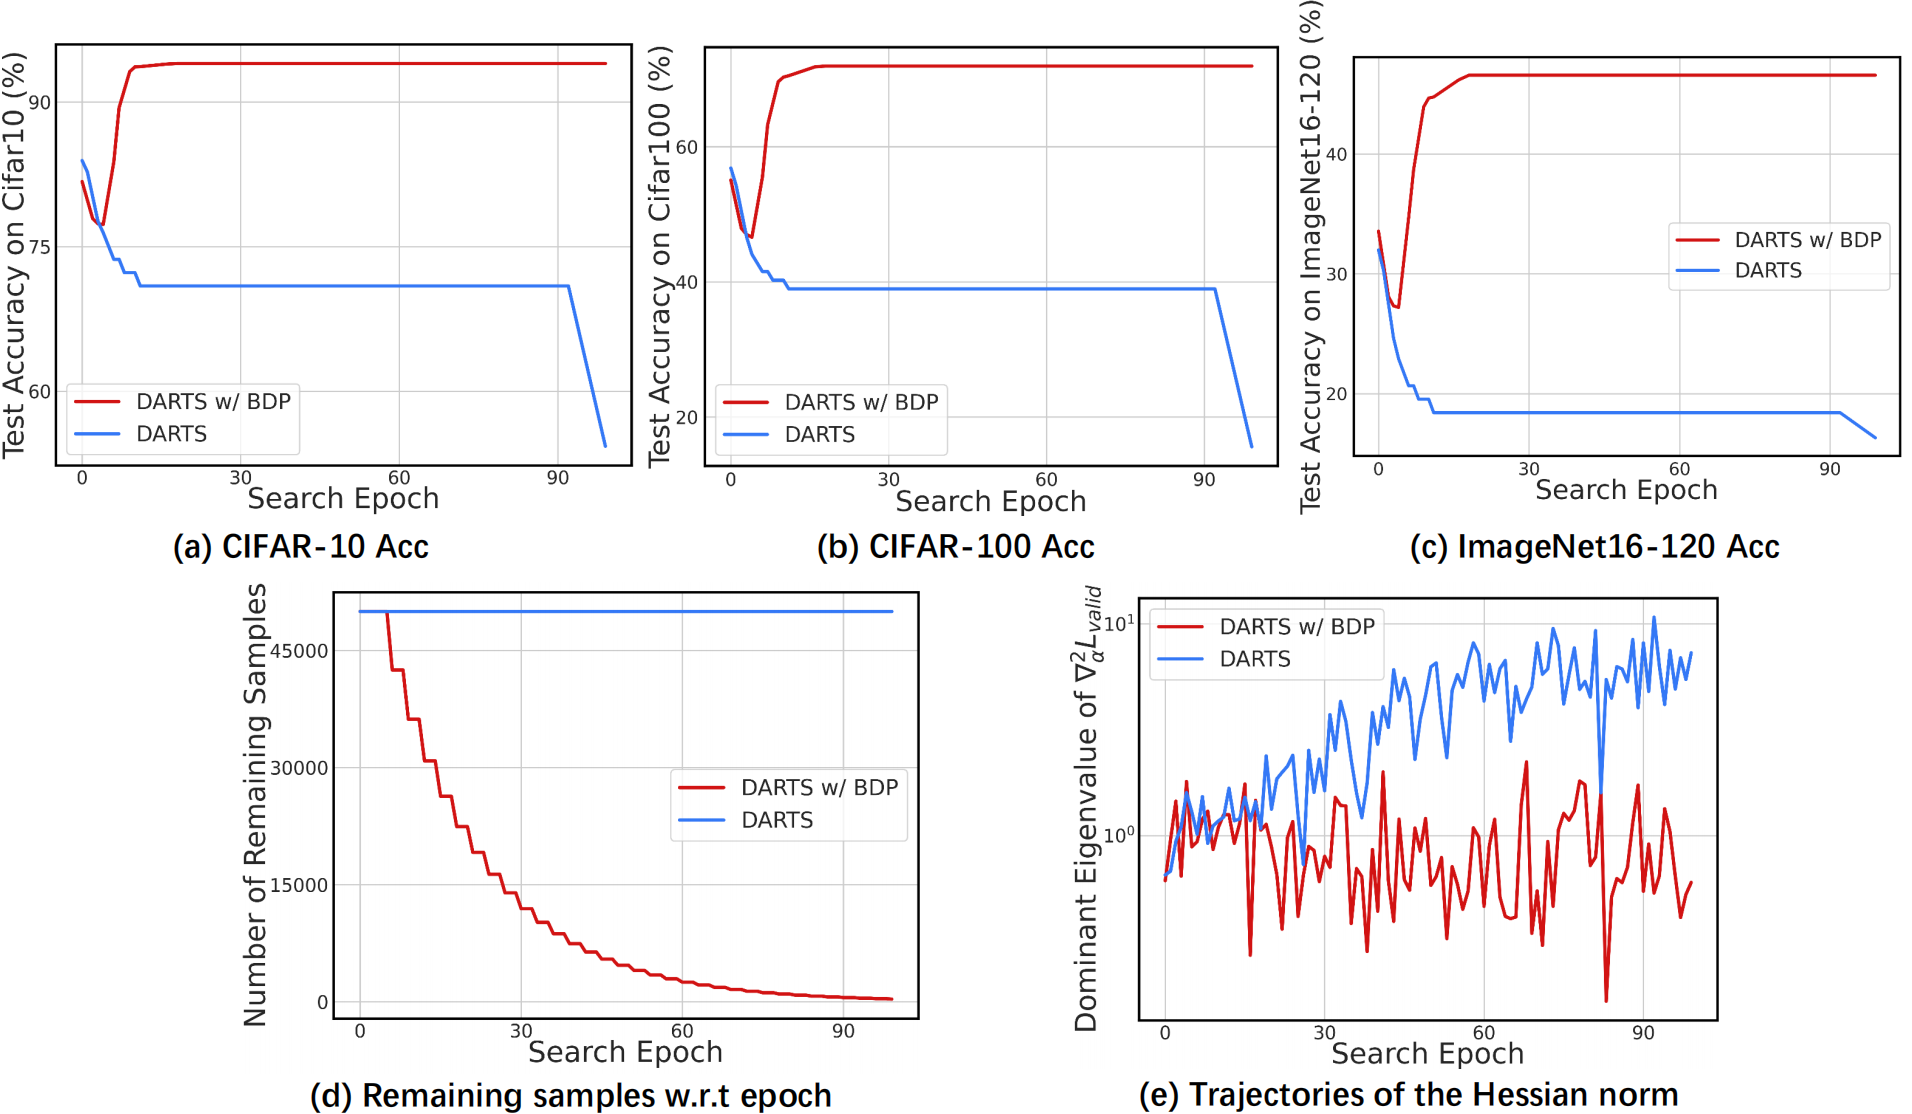} 
	\caption{
         More comparisons of DARTS and DARTS w/ BDP search process on NAS-Bench-201~\cite{dong2020bench} on the CIFAR-10 dataset. (a)-(c) Test accuracies on CIFAR-10, CIFAR-100 and ImageNet16-120; (d) Number of remaining samples; (e) Trajectories of the dominant eigenvalues of $\nabla^{2}_{\alpha}L_{valid}$.  
         For DARTS, the performance rapidly collapses on all test datasets, the number of samples remains unchanged, and the dominant eigenvalue persistently increases. For DARTS w/ BDP, the performance gradually increases, the number of samples gradually decreases, and the dominant eigenvalue oscillates down.
 } \vspace{-2mm}
	\label{fig: bench_change_C10}
\end{figure*}
\begin{figure*}[htbp] 
	\centering 
	\includegraphics[width=0.86\linewidth]{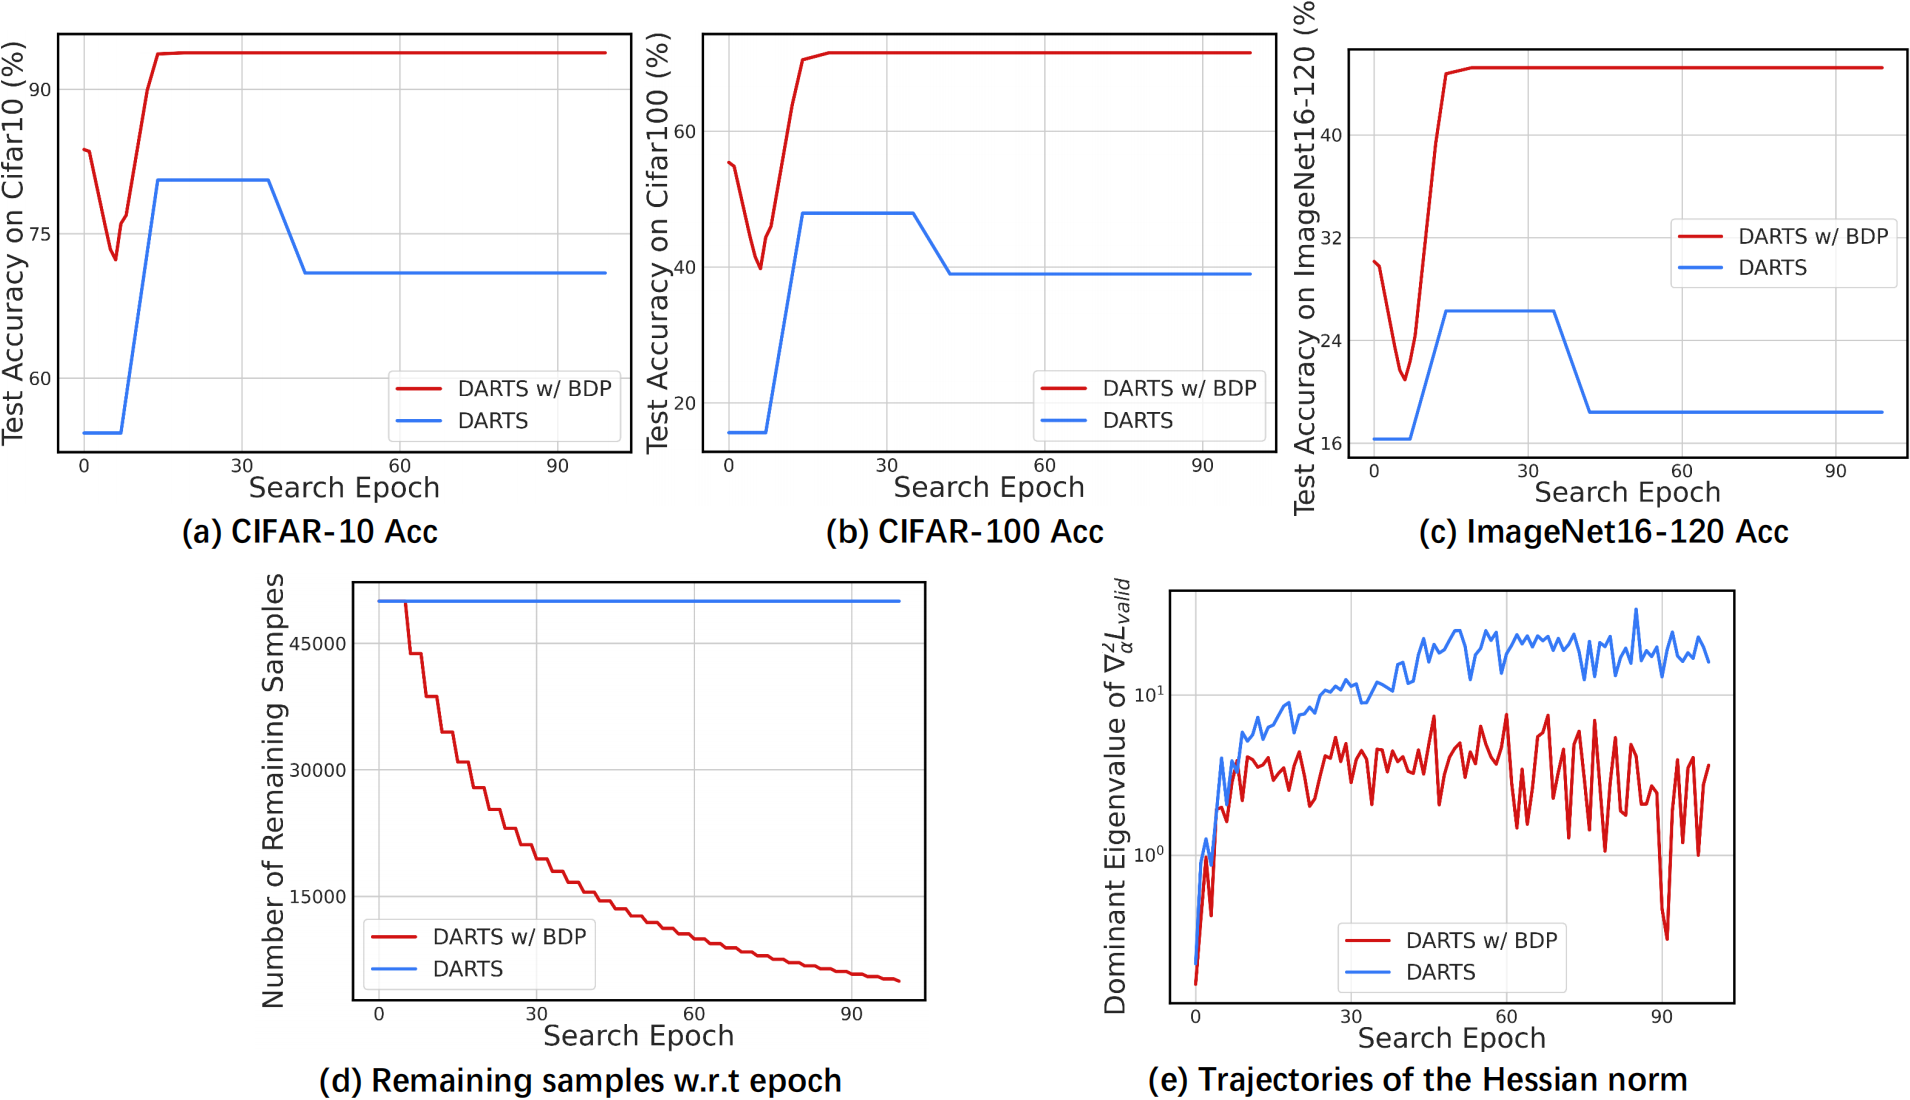} 
	\caption{
         More comparisons of DARTS and DARTS w/ BDP search process on NAS-Bench-201~\cite{dong2020bench} on the CIFAR-100 dataset. (a)-(c) Test accuracies on CIFAR-10, CIFAR-100 and ImageNet16-120; (d) Number of remaining samples; (e) The trajectories of the dominant eigenvalues of $\nabla^{2}_{\alpha}L_{valid}$.  
         For DARTS, the performance rapidly collapses on all test datasets, the number of samples remains unchanged, and the dominant eigenvalue persistently increases. For DARTS w/ BDP, the performance gradually increases, the number of samples gradually decreases, and the dominant eigenvalue oscillates down after the early stage of training.
 } \vspace{-2mm}
	\label{fig: bench_change_C100}
\end{figure*}

\subsection{Effectiveness of the Class Balance Constraint}
\label{sec: appendix: balance}
Then,~\cref{fig: class_num_C10}
% and ~\cref{fig: class_num_C100} 
show the impact of class balance constraint on DARTS w/ BDP. Subgraphs (a)-(c) shows the changes in the number of samples of each class at three training stages with and without class balance constraints. We can see that if there is no class balance constraint, 
some classes in the dataset will be pruned most or even all samples in the early or mid-term of training, while some other classes still have many samples left. In short, the class imbalance in the dataset is very severe. As a comparison, in the search process with the constraints, the number of samples between different classes is more balanced. 
% Only in the later stage of training will the samples of a specific class be all pruned. 
This shows that the proposed class balance constraint is reasonable and necessary for BDP. Note that our aim is not to achieve complete class balance, which means a moderate difference in the number of samples between different classes is acceptable. 

In addition, we find that in a dataset with a small number of total classes, such as CIFAR-10, BDP without the class balance constraint will only cause a slight class imbalance and have a small impact on performance. 
While in a dataset with a large number of total classes, such as CIFAR-100, BDP without the class balance constraint may cause severe class imbalance, which will cause relatively large interference to performance. 
This can be concluded from the results of our main text's ablation experiment ~\cref{tab:ablation: balance}. Specifically, without the class balance constraint, DARTS w/ BDP has only a 0.3\% performance degradation on CIFAR-10 but a serious performance degradation of nearly 4.5\% on CIFAR-100 on the NAS-Bench-201 benchmark~\cite{dong2020bench}.

\begin{figure*}[htbp] 
	\centering 
	\includegraphics[width=0.95\linewidth]{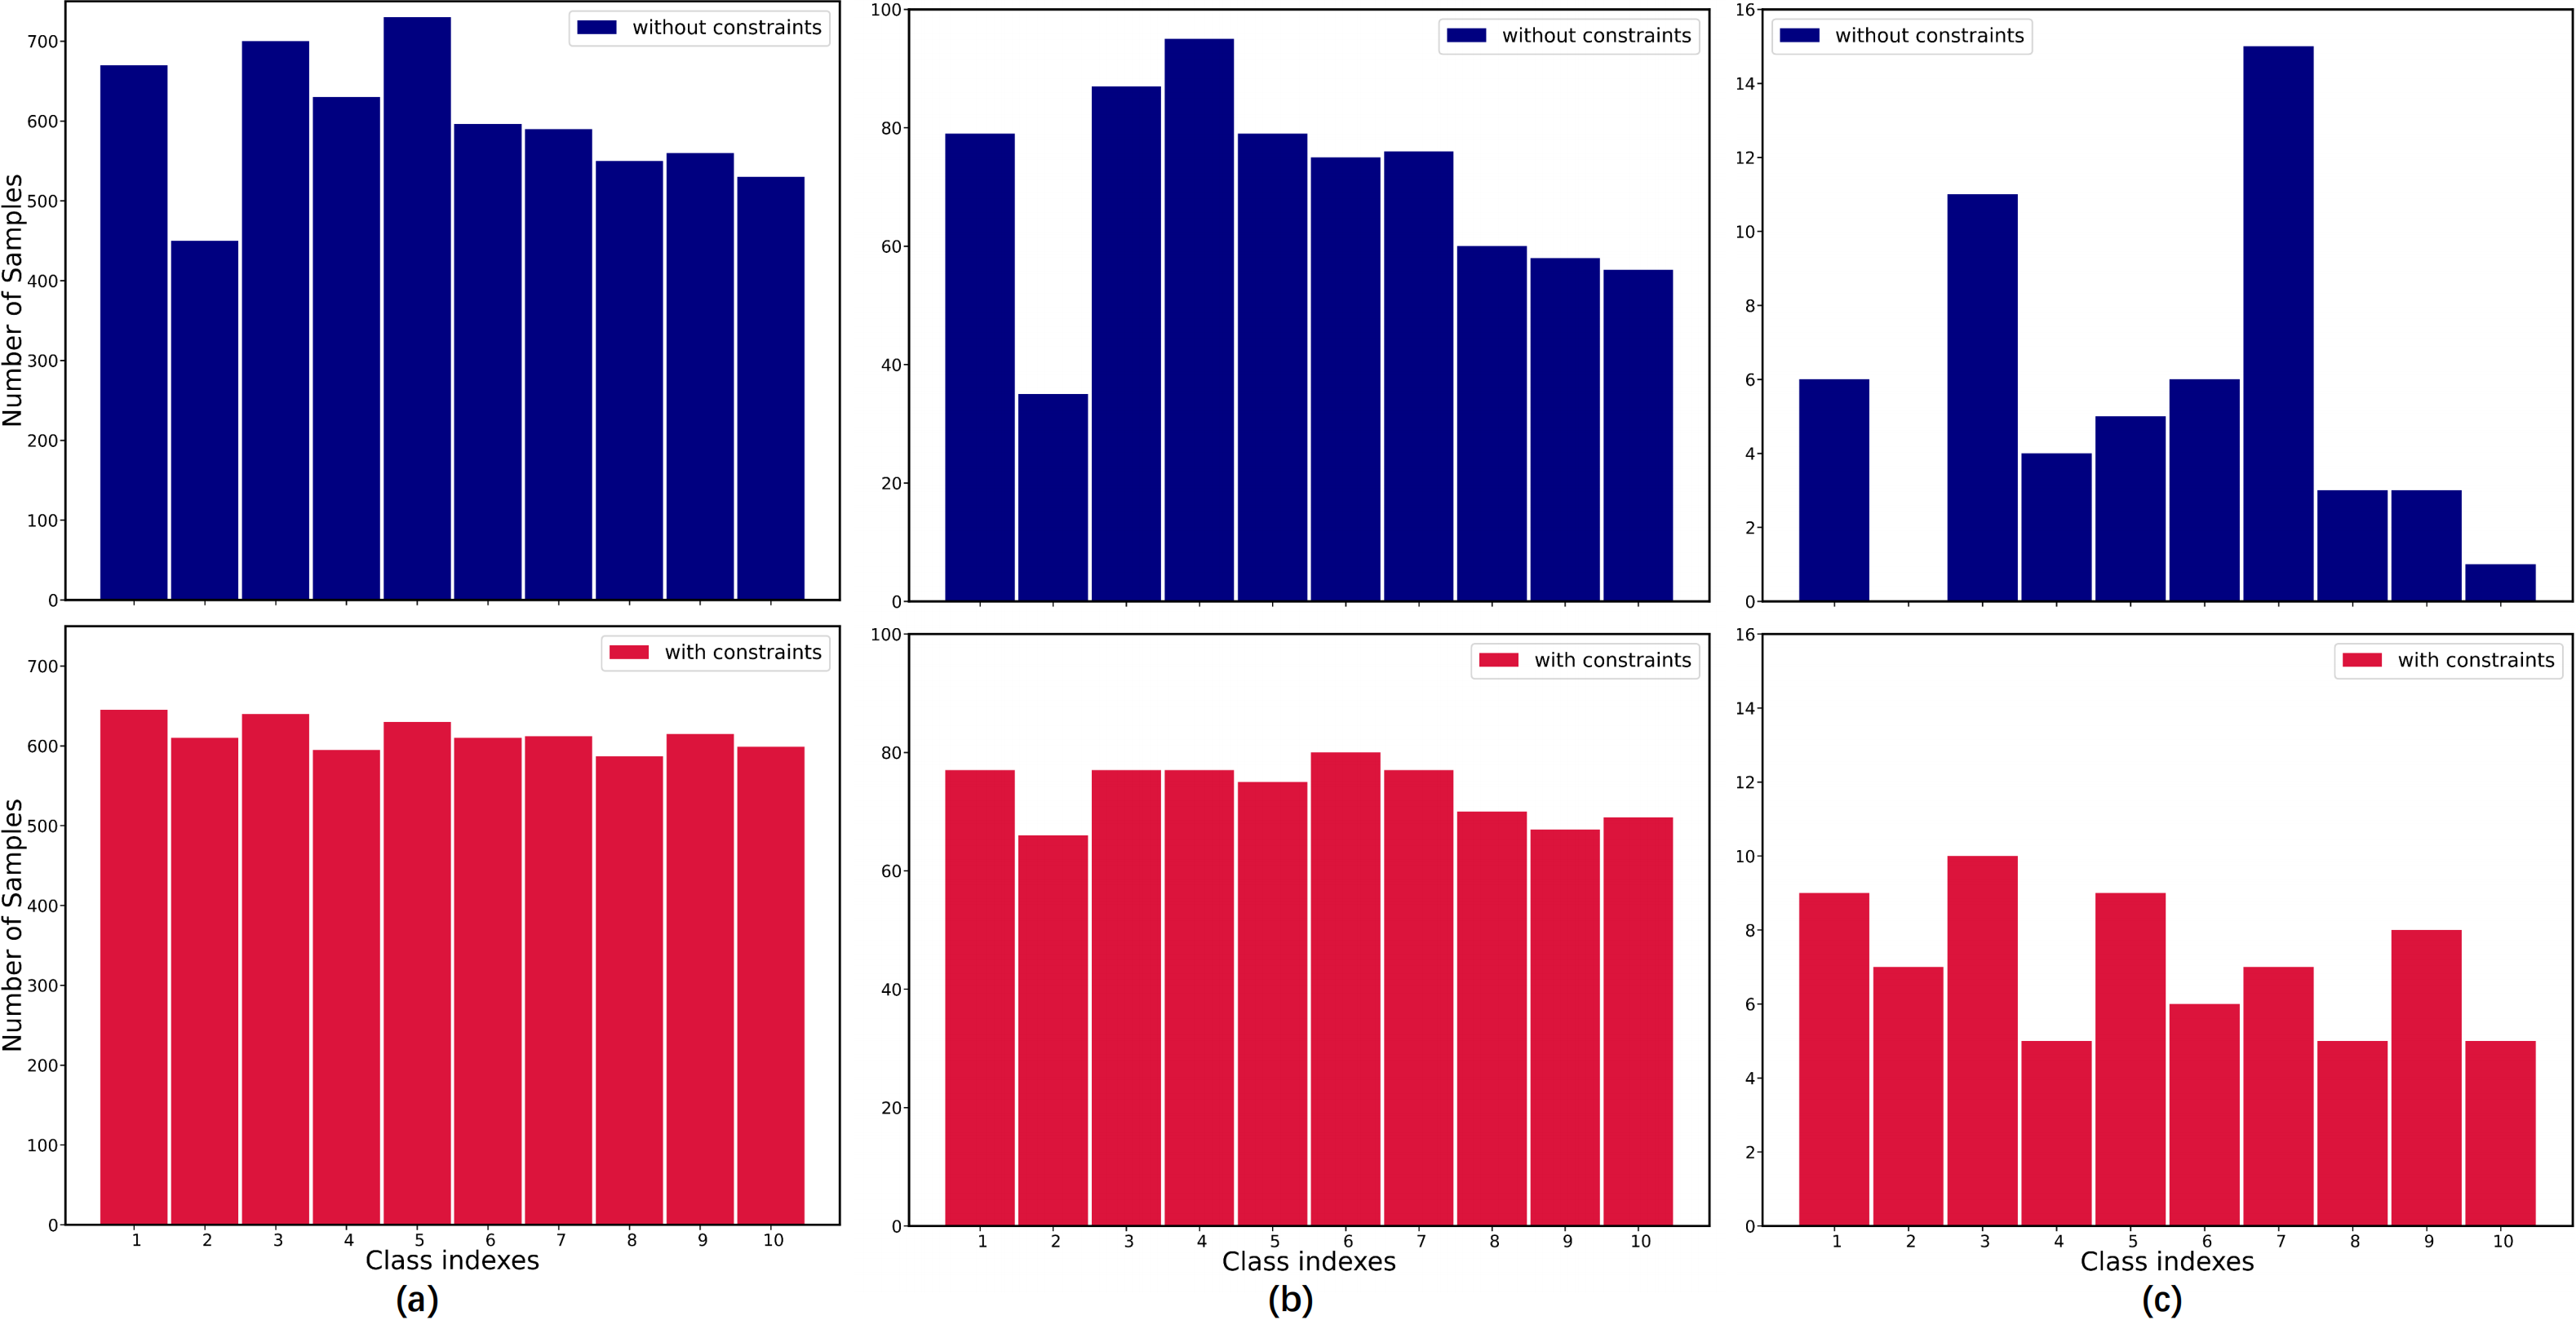} 
	\caption{Comparison between DARTS w/ BDP with and without class balance constraint at different training epochs. The experiments are conducted on CIFAR-10 on NAS-Bench-201~\cite{dong2020bench}. Let $E$ denote the total training epochs. (a), (b), and (c) show the number of remaining samples of each class in the dataset at the $\frac{E}{3}$, $\frac{2E}{3}$, and $E$ epochs respectively. Each vertical bar represents the number of samples in a class, and the horizontal axis represents the index of all classes in the dataset.
 } \vspace{-2mm}
	\label{fig: class_num_C10}
\end{figure*}

\subsection{Comparisons of Different Kinds of Class Balance Constraints}
We use class balance constraints of different functional forms for DARTS w/ BDP for comparisons. Let $b$ denote the balance degree of the dataset and $N$ denote the intensity of the class balance constraint. The compared constraints all meet three requirements: 1) If the classes are perfectly balanced, \ie, $b$ = 1; thus $N$ = 1, there is no constraints; 2) With the pruning of data, class imbalance gradually emerges, resulting in the decrease of $b$ and, therefore, $N$ increases to suppress the class imbalance from becoming too severe. 3) When $b$ is close to 0, $N$ will be relatively large. The increased $N$ will keep classes with fewer samples from being further pruned and exert a tendency to prune classes with more samples, thus compensating for class imbalance. 

We perform experiments on the CIFAR-100 dataset on NAS-Bench-201 for more visible performance differences. The comparisons are shown in~\cref{tab: appendix: different constraint}. 
According to the results in the table, we can draw the conclusion that as $b$ decreases, it is better to have a relatively uniform and appropriate rising speed of $N$ as seen in constraints (a), (b), (d), and (e). These types of constraints positively impact the performance. 
Conversely, when using constraints (c) and (f), the value of $N$ increases too rapidly as soon as $b$ starts to decrease from 1. This causes the constraint to become excessively strong and results in unstable performances. 

\iffalse
\begin{table}[htbp]
\centering
\caption{Results of different functional forms of class balance constraints. For each constraint, three experiments are conducted using three different random seeds on the CIFAR-10 and CIFAR-100 on NAS-Bench-201 benchmark~\cite{dong2020bench} "Original" represents the class balance constraint used in the original paper. (a)-(c) correspond to the listed constraints above respectively.}
\vspace{2mm}
\label{tab: appendix: different constraint}
\vspace{-3mm}
\setlength{\tabcolsep}{1.8mm}
\resizebox{1.0\linewidth}{!}{
\begin{tabular}{ccccc}
\toprule
\multirow{2}{*}{Constraints} & \multicolumn{2}{c}{CIFAR-10} & \multicolumn{2}{c}{CIFAR-100} \\ 
\cmidrule(lr){2-5} 
                             & valid         & test         & valid         & test          \\ 
\midrule
No constraint                   & 90.68\pm0.37  & 93.66\pm0.52      & 67.27\pm3.03  & 66.43\pm3.44     \\
Original                     & 90.98\pm0.24    & 93.79\pm0.39   & 71.61\pm0.74    & 71.64\pm1.30    \\
(a)                            & 90.77\pm0.23    & 93.73\pm0.09   & 70.57\pm1.27    & 70.09\pm1.21    \\
(b)                            & 89.76\pm2.47    & 92.63\pm2.06   & 66.62\pm5.89    & 66.52\pm5.27    \\
(c)                            & 90.63\pm0.20    & 93.57\pm0.09   & 62.06\pm12.92   & 63.72\pm9.97   \\ 
\bottomrule
\end{tabular}}
\vspace{-5mm}
\end{table}
\fi

\begin{table}[htbp]
\centering
\caption{Comparisons of class balance constraints of different functional forms. For each constraint, 5 experiments are conducted using different random seeds on NAS-Bench-201~\cite{dong2020bench} on CIFAR-100. Index (a) represents the constraint used in our main text. (b)-(f) correspond to the compared constraints.}
\vspace{2mm}
\label{tab: appendix: different constraint}
\vspace{-3mm}
\resizebox{0.9\linewidth}{!}{%
\setlength{\tabcolsep}{3mm}
\begin{tabular}{ccc}
\toprule
Index & Constraints  &  CIFAR-100  Acc \\ 
\cmidrule(lr){1-3}
- & $N=1$ \textit{(no constraints)}  & 66.43\pm3.44     \\
(a) & $N = n\left(1-b^{2}\right)+1$     & 71.64\pm1.30    \\
(b)&   $ N = n^{1-b}$             & 70.21\pm1.21    \\
(c)& $N=e^{n(1-b)}$     & 58.26\pm12.01 \\
(d)& $1-n\log b$        & 66.97\pm 2.76 \\
(e)&   $N = n\left(1-b\right)+1$             & 66.52\pm5.27    \\
(f)&   $N = n\left(1-b^{3}\right)+1$             & 63.72\pm9.97   \\ 

\bottomrule
\end{tabular}}
\vspace{-3mm}
\end{table}

\subsection{Details of Data Pruning Strategy}
As illustrated in \cref{sec: method pruning strategy} of the main text, we conduct comprehensive experiments on the NAS-Bench-201 benchmark to explore the optimal data pruning criterion for DARTS. For each criterion, we set multiple pruning ratios (\ie, $(p_t/p_v)\%=[(25/5), (20/10), (15/15), (10/20), (5/25)]$) for the training and validation sets and record the results in \cref{tab: criterion}. As can be concluded, the criterion \textbf{Low \& High} provides the best performance, which means pruning samples with the lowest VoE scores from the training set and pruning samples with the highest VoE scores from the validation set.

\begin{table*}[h]
\centering
\caption{
Detailed results of data pruning strategy exploration the NAS-Bench-201 benchmark~\cite{dong2020bench}. \textbf{Low} means pruning samples with the lowest VoE scores from the dataset while \textbf{High} means the opposite.
Five pruning ratios $(p_t/p_v)\%=[(25/5), (20/10), (15/15), (10/20), (5/25)]$ are applied to each criterion.
The highest accuracy of each dataset is \textbf{bolded}.
}
\label{tab: criterion}
\vspace{-3mm}
\setlength{\tabcolsep}{1.8mm}
\resizebox{1.0\linewidth}{!}{
\begin{tabular}{cc ccccc ccccc ccccc}
\toprule
\multicolumn{2}{c}{Criterion} & \multicolumn{5}{c}{CIFAR-10} & \multicolumn{5}{c}{CIFAR-100} & \multicolumn{5}{c}{Img.16-120}\\
\cmidrule(lr){1-2} \cmidrule(lr){3-7} \cmidrule(lr){8-12} \cmidrule(lr){13-17}    
{$T$}  & {$V$}    & {25/5} & {20/10} & {15/15} & {10/20} & {5/25} & {25/5} & {20/10} & {15/15} & {10/20} & {5/25} & {25/5} & {20/10} & {15/15} & {10/20} & {5/25} \\
\cmidrule(lr){1-2} \cmidrule(lr){3-7} \cmidrule(lr){8-12} \cmidrule(lr){13-17} 
\textbf{Low}  & \textbf{Low}  & 54.30 & 54.30 & 54.30 & 54.30 & 54.30 & 15.61 & 15.61 & 15.61 & 15.61 & 64.34 & 16.32 & 16.32 & 16.32 & 16.32 & 16.32 \\
\textbf{Low}  & \textbf{High} & \textbf{93.62} & 90.25 & 54.30 & 80.57 & 88.32 & \textbf{72.99} & 64.34 & 68.76 & 60.02 & 61.12 & \textbf{44.57} & 40.10 & 16.32 & 26.29 & 33.67 \\
\textbf{High} & \textbf{Low} & 54.30 & 54.30 & 54.30 & 70.92 & 54.30 & 15.61 & 38.97 & 63.52 & 34.37 & 48.12 & 16.32 & 16.32 & 16.32 & 18.41 & 16.32 \\
\textbf{High} & \textbf{High} & 54.30 & 54.30 & 54.30 & 80.57 & 90.36 & 15.61 & 15.61 & 15.61 & 15.61 & 15.61 & 16.32 & 16.32 & 16.32 & 26.29 & 38.59 \\
\bottomrule
\end{tabular}}
\vspace{-3mm}
\end{table*}

\section{Visualization of the Searched Architectures}
\label{sec: appendix: cell structure}
\subsection{DARTS Search Space}
In ~\cref{fig: cell structure}, we visualize the normal cell and reduction cell searched by DARTS and DARTS w/ BDP on the DARTS search space. Compared with (a), the searched architectures of (b) and (c) have fewer parameter-free operations, such as skip-connection and max-pooling. 
This is beneficial to preventing the performance degradation of the searched architecture and thus obtaining better results. 
We also visualize the searched architectures by applying BDP to DARTS variants in ~\cref{fig: cell structure variants}.

\subsection{MobileNet Search Space}
We provide the visualization of the searched architectures on the MobileNet-like search space, a chain-structured search space. The results are shown in ~\cref{fig: cell structure mobile}. 

\begin{figure*}[htbp] 
	\centering 
	\includegraphics[width=0.85\linewidth]{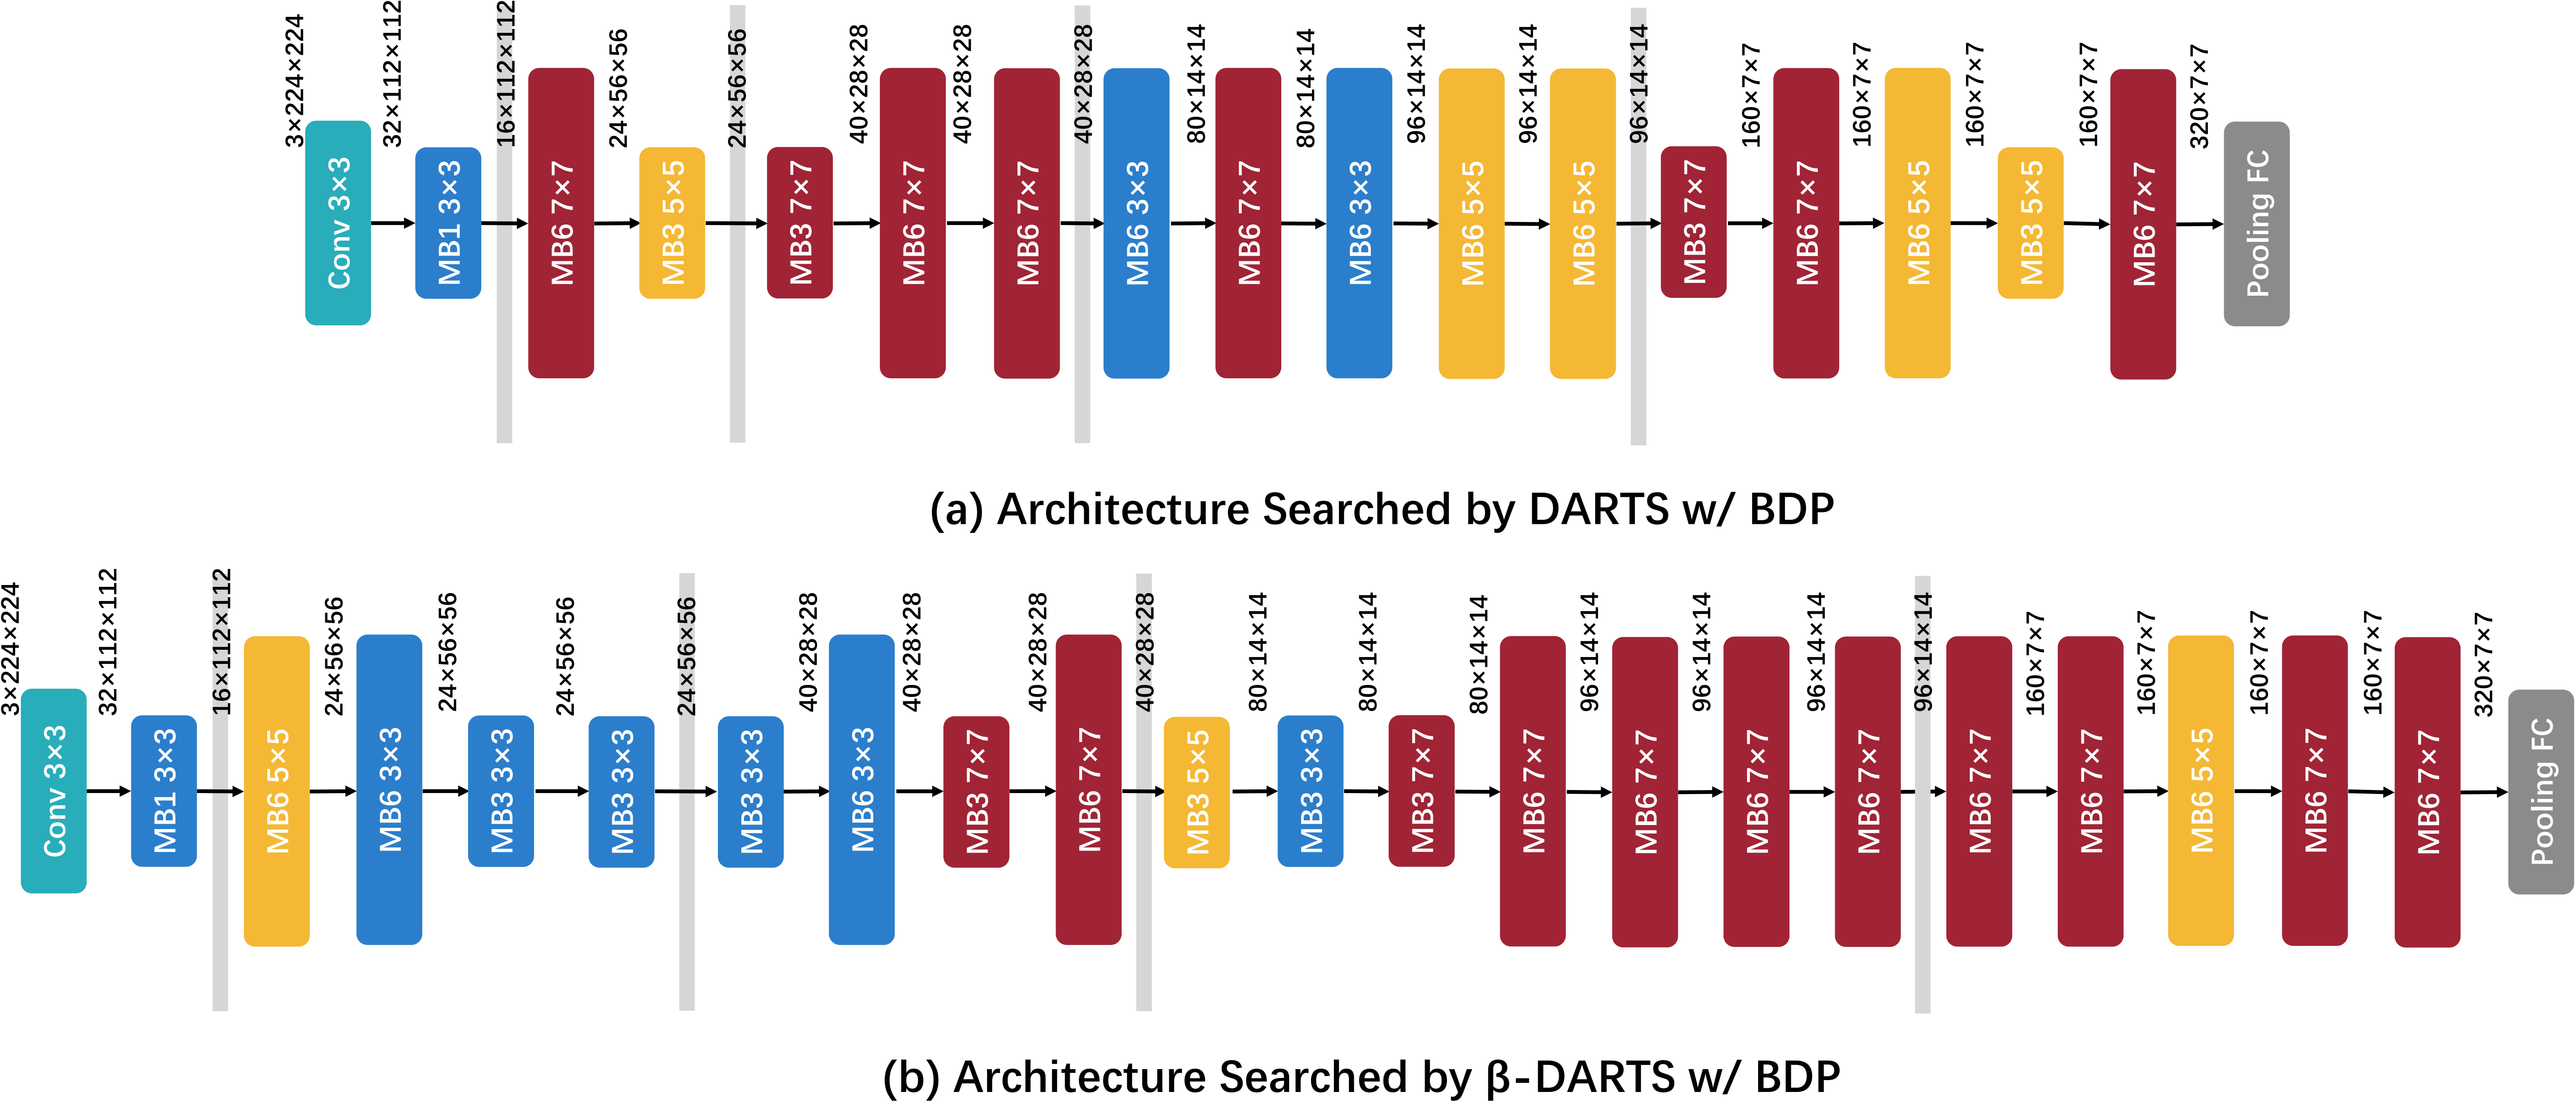} 
	\caption{
The searched architecture by DARTS w/ BDP (a) and $\beta-$DARTS w/ BDP (b) on MobileNet-like search space on the ImageNet dataset. $3\times3$, $5\times5$ and $7\times7$ are kernel sizes of convolutions, and
MB3(6) denotes an inverted bottleneck convolution layer with an expansion ratio of 3(6). 
 } \vspace{-2mm}
	\label{fig: cell structure mobile}
\end{figure*}

\begin{figure*}[htbp] 
	\centering 
	\includegraphics[width=0.85\linewidth]{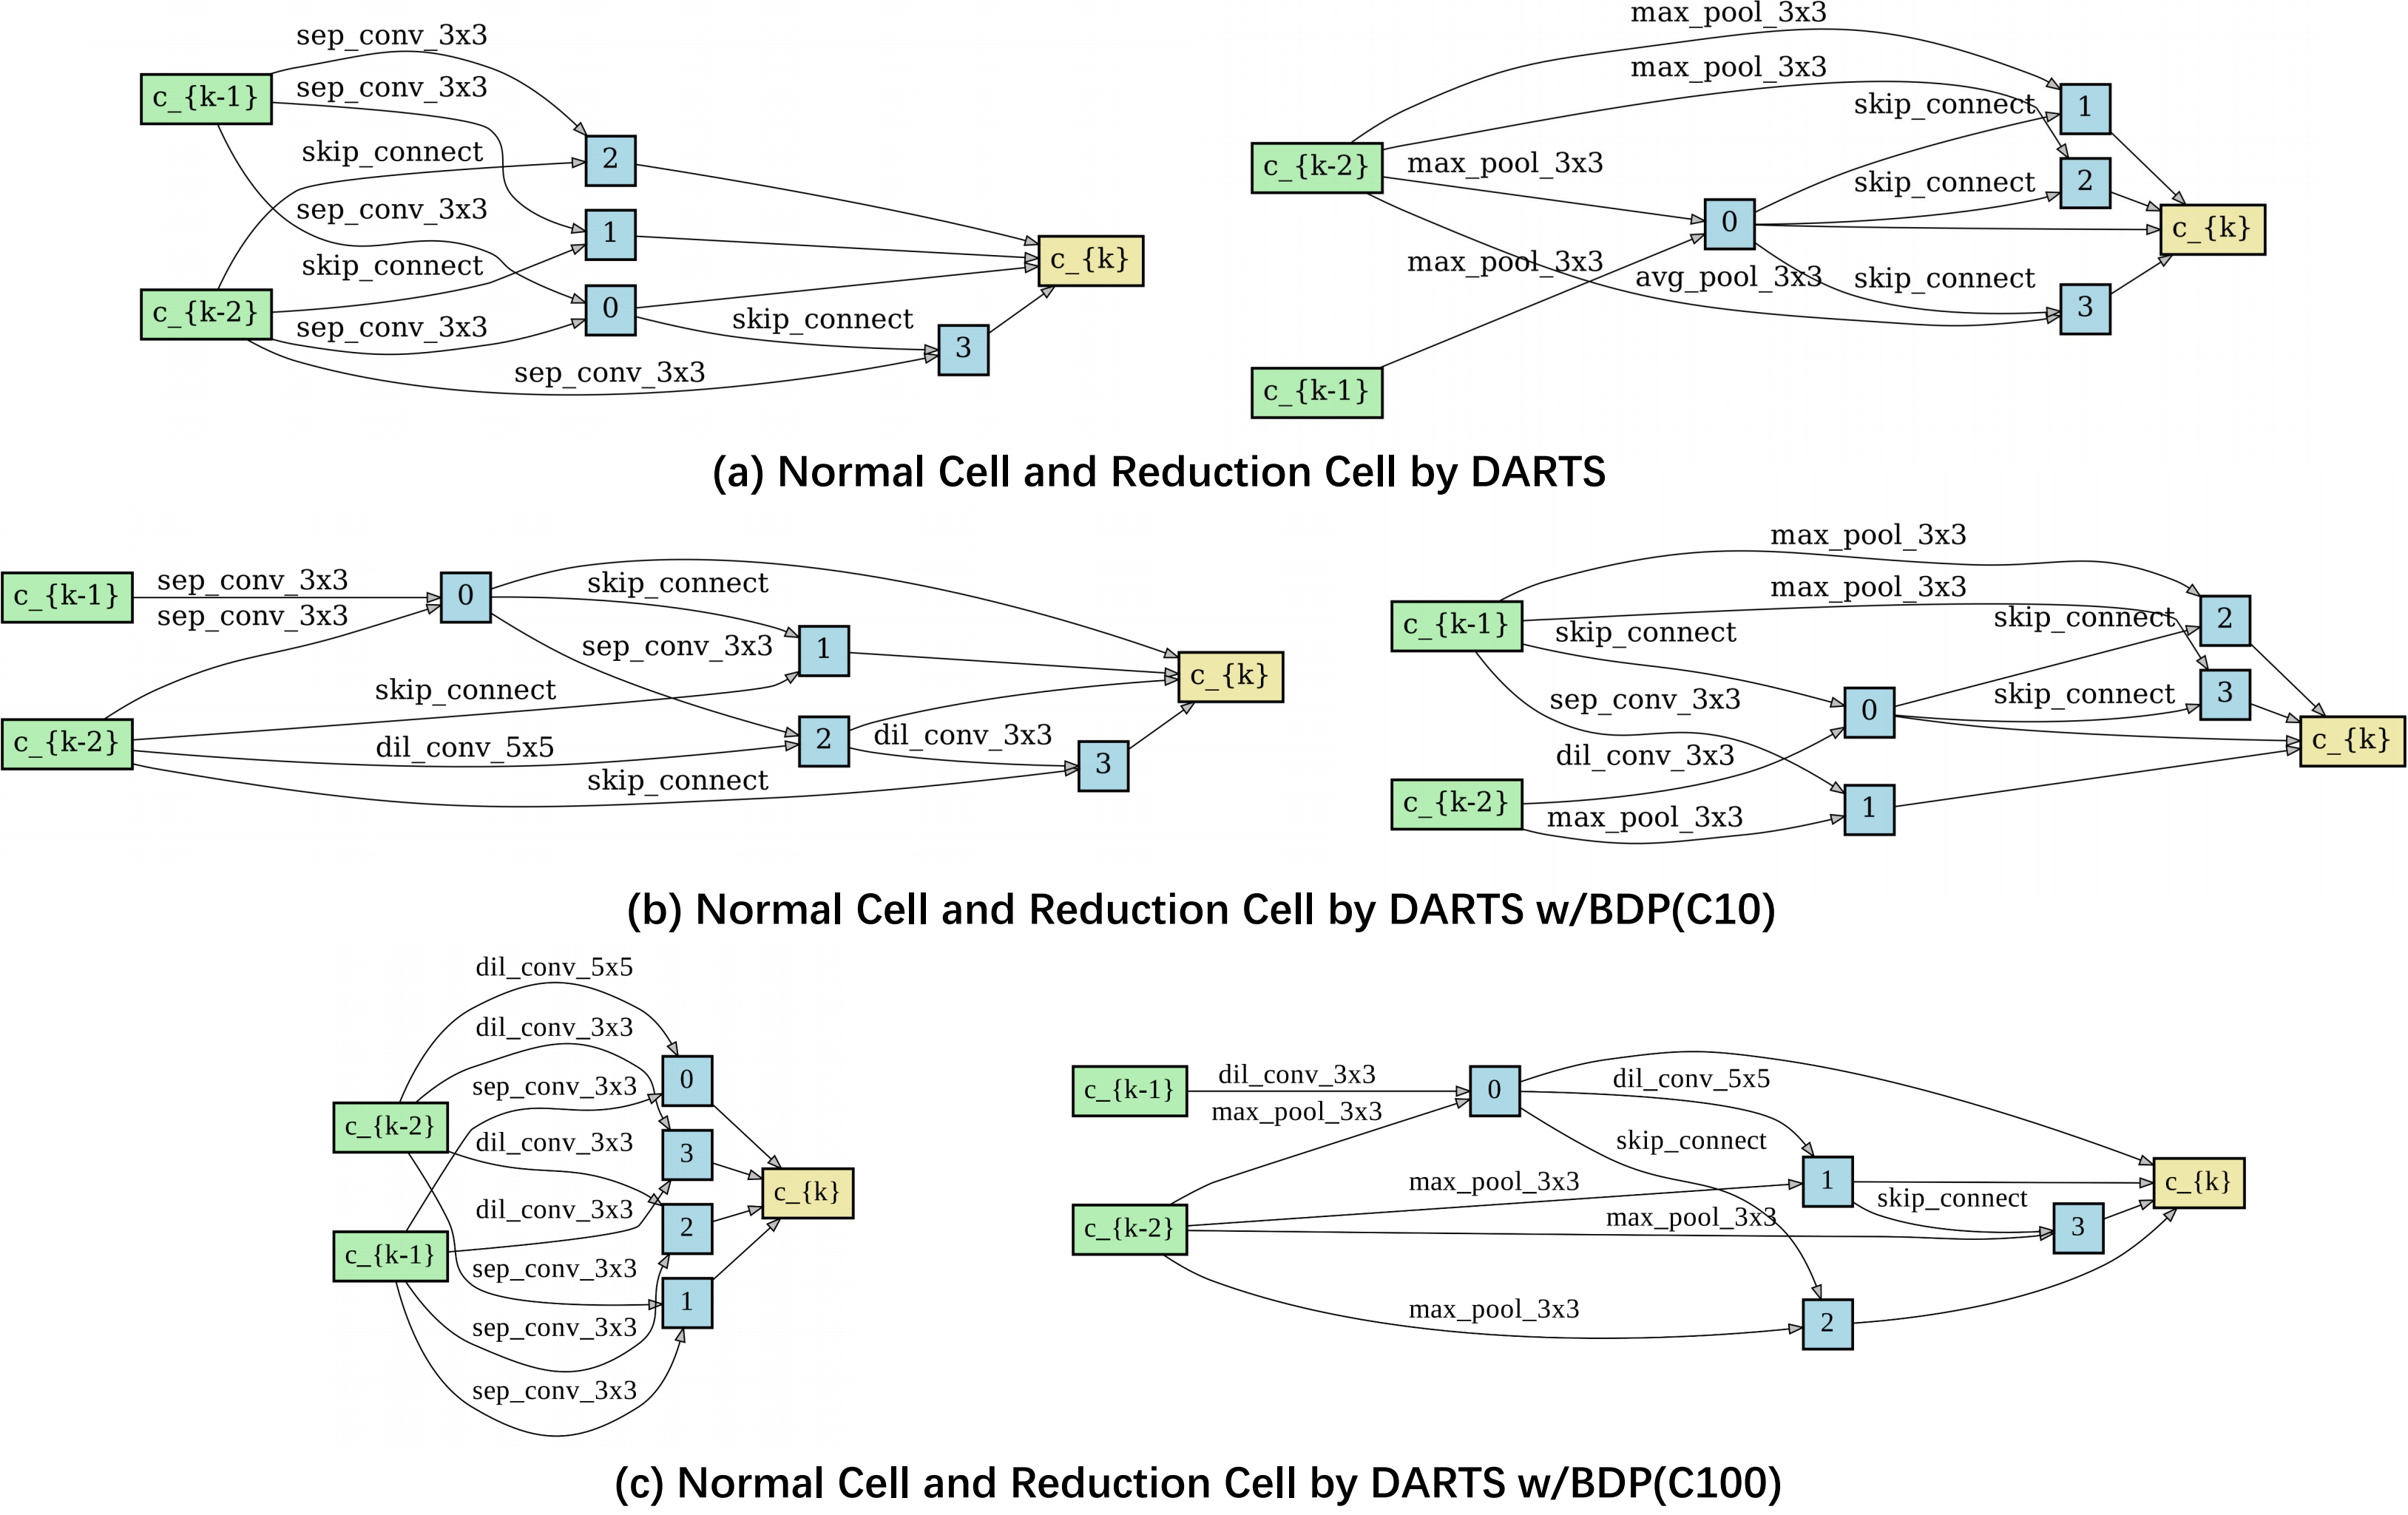} 
	\caption{Normal cell (left) and Reduction cell (right) found by DARTS and DARTS w/ BDP on the DARTS search space. (a) is the reported architecture of DARTS~\cite{liu2018darts}. (b) and (c) denote the searched genotypes by DARTS w/ BDP on CIFAR-10 and CIFAR-100.
 } \vspace{-2mm}
	\label{fig: cell structure}
\end{figure*}

\begin{figure*}[htbp] 
	\centering 
	\includegraphics[width=0.85\linewidth]{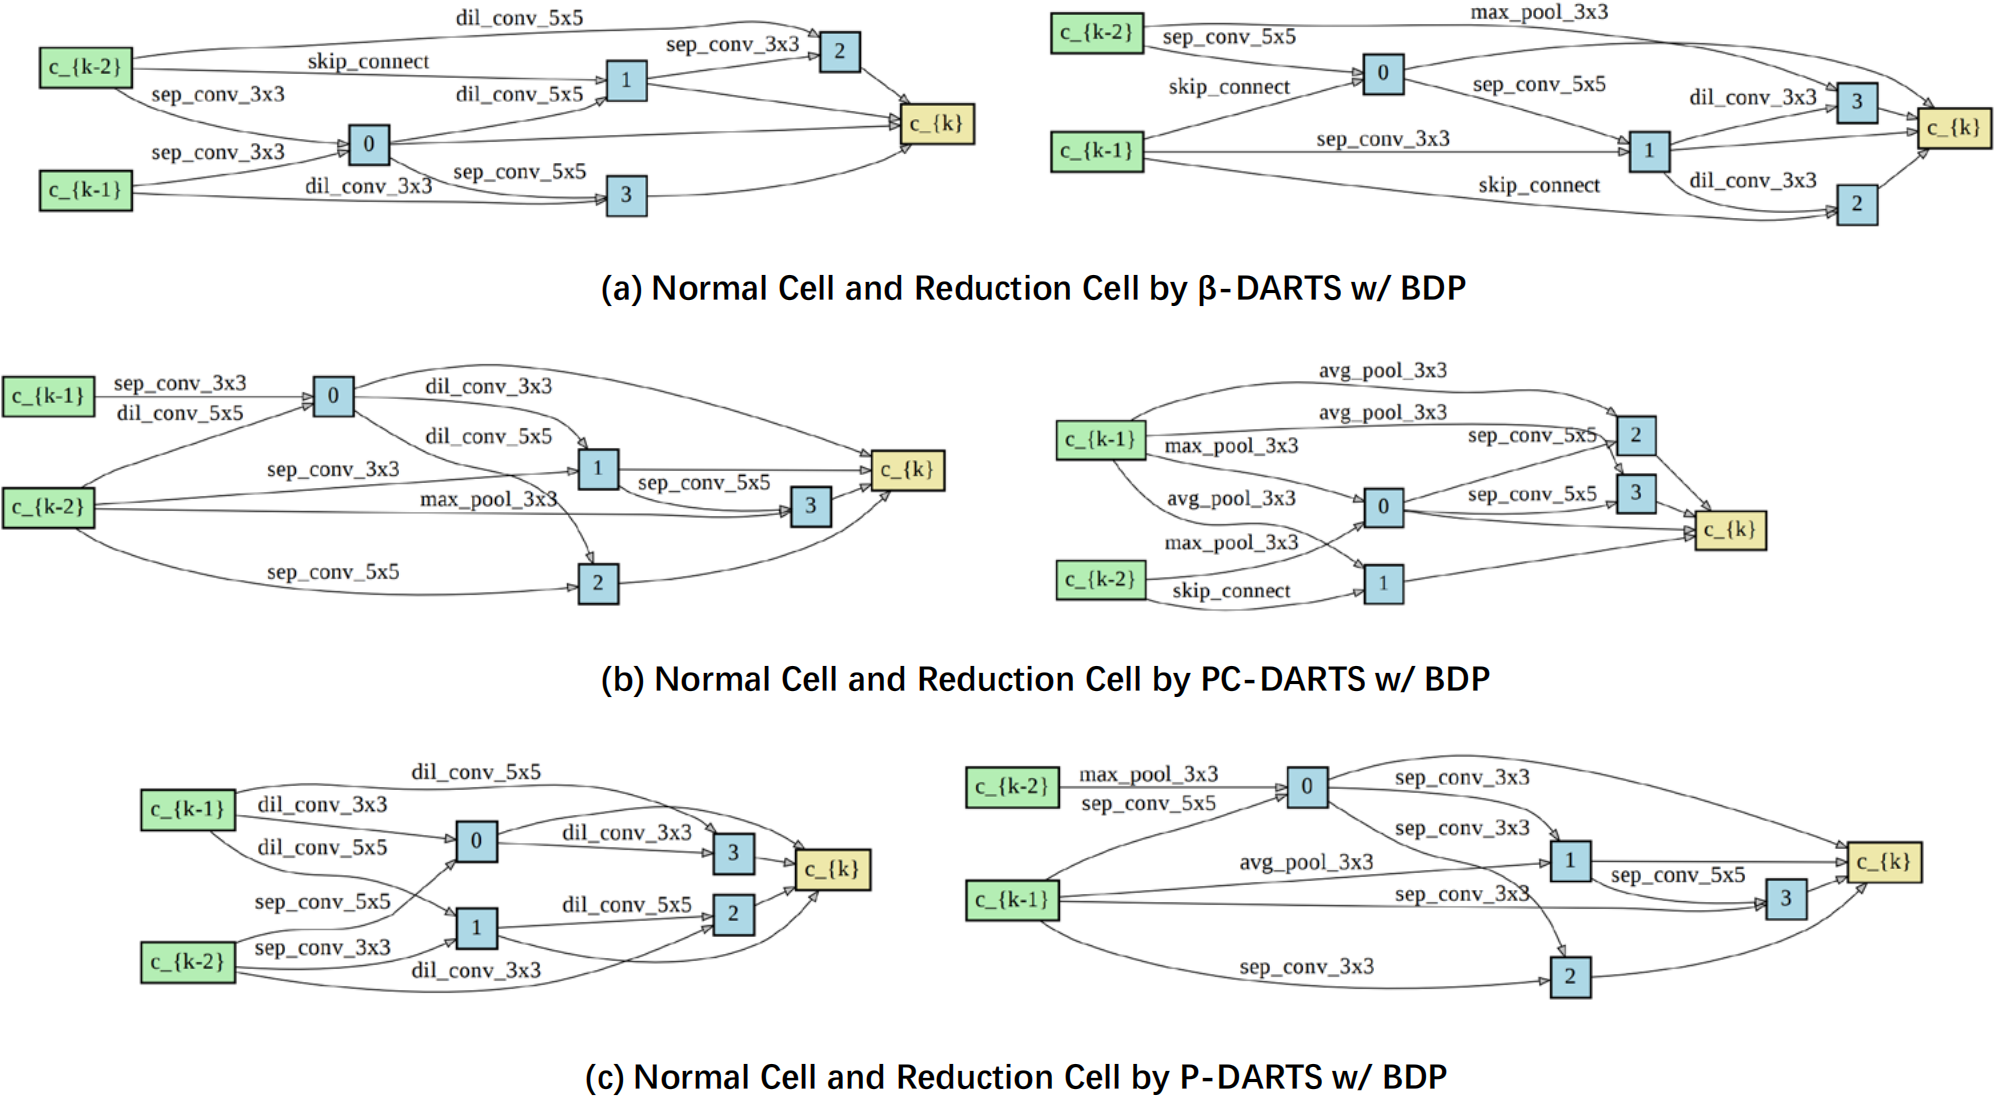} 
	\caption{Normal cell (left) and Reduction cell (right) found by DARTS variants w/ BDP on the DARTS search space.
 } \vspace{-2mm}
	\label{fig: cell structure variants}
\end{figure*}

\section{Limitations and Future Works}
\iffalse
% 需要改完之后重写一下
The BDP algorithm proposed in this paper only targets a specific mainstream of NAS, namely differentiable architecture search (DARTS). From the results and findings of this paper, data pruning algorithms have great potential in the field of one-shot NAS and are almost unexplored. In addition, as one of the pioneer explorations of designing data-efficient algorithms based on the characteristics of architecture search methods, the data pruning indicator and class balance problem handling (which are also essential and less explored in data pruning) still need more optimization. Future research will explore more general data pruning algorithms for one-shot NAS methods. At the same time, we also hope that the observation and exploration of this paper from the data perspective to improve the efficiency of DARTS further can attract the community’s attention and research on this important topic of reducing the cost of neural architecture search from the data perspective. 
\fi
The BDP paradigm proposed in this paper focuses on differentiable architecture search (DARTS), which is a specific mainstream of NAS. However, this paper's results suggest that data pruning algorithms have great potential in the field of one-shot NAS and are currently under-explored. As one of the pioneer studies on designing data-efficient algorithms for architecture search methods, this paper highlights the need for more efforts and refinements in the data-efficient algorithms and class balance problem handling, which are also essential but less explored. A promising future research topic is exploring more general data-efficient algorithms for one-shot NAS methods.

\iffalse
\section{Rationale}
\label{sec:rationale}
% 
Having the supplementary compiled together with the main paper means that:
% 
\begin{itemize}
\item The supplementary can back-reference sections of the main paper, for example, we can refer to \cref{sec:intro};
\item The main paper can forward reference sub-sections within the supplementary explicitly (e.g. referring to a particular experiment); 
\item When submitted to arXiv, the supplementary will already included at the end of the paper.
\end{itemize}
% 
To split the supplementary pages from the main paper, you can use \href{https://support.apple.com/en-ca/guide/preview/prvw11793/mac#:~:text=Delete%20a%20page%20from%20a,or%20choose%20Edit%20%3E%20Delete).}{Preview (on macOS)}, \href{https://www.adobe.com/acrobat/how-to/delete-pages-from-pdf.html#:~:text=Choose%20%E2%80%9CTools%E2%80%9D%20%3E%20%E2%80%9COrganize,or%20pages%20from%20the%20file.}{Adobe Acrobat} (on all OSs), as well as \href{https://superuser.com/questions/517986/is-it-possible-to-delete-some-pages-of-a-pdf-document}{command line tools}.
\fi
